# Supplementary material for: Superquantile-based learning: a direct approach using gradient-based optimization
Source: arXiv:2201.00505 source file (2022-01-03)
Supplement: Supplementary file 1 [file appendix.tex]

%===================================================================
%===================================================================
\section{Proof of Theorem\texorpdfstring{\;\ref{thm:uniform-convergence-param}}{}} \label{sec:a:gen_bound}
%===================================================================
%===================================================================

In this appendix, we provide a complete proof of Theorem\;\ref{thm:uniform-convergence-param}. For classical results in this spirit, we refer to the monograph \cite{zbMATH05133436}. 
For discussions on statistical aspects of statistical learning, we refer to \eg\cite{DBLP:journals/corr/abs-1810-08750,mhammedi2020pac,lee2020learning}. 

%\begin{proof}
 
    The key step in the proof of Theorem\;\ref{thm:uniform-convergence-param} is to show the uniform convergence 
    \begin{equation}\label{eq:key}
    \text{$\Rpn(w) \to \Rp(w)$ almost surely for all $w \in W$.} 
    \end{equation}
    Indeed, once we have this, 
    the result immediately follows as
	\begin{align}
		0 \le \Rp(w_n^\star) - \Rp(w^\star)
		&= 
		\Rp(w_n^\star) - \Rpn(w_n^\star)
		+ \Rpn(w_n^\star) - \Rpn(w^\star)
		+ \Rpn(w^\star) - \Rp(w^\star)\\
		&\le 
		2 \sup_{w \in W} |\Rpn(w) - \Rp(w)|
		\to 0,
	\end{align}
	%almost surely, 
	where we use $\Rpn(w_n^\star) \le \Rpn(w^\star)$ in the second inequality.

	In order to prove~\eqref{eq:key}, %the uniform convergence above, 
	we use the variational expression of the superquantile\;\eqref{eq:def_min_cvar}. 
	We define 
	\[
		\bar \Rp(w, \eta)
		= \eta + \frac{1}{1-p} \mathbb{E}_{(x, y)\sim P}
		[\max(\ell(y, \varphi(w, x))-\eta,0)] \,,
	\]
	so that, using that the loss is bounded by $B$, we can write
	\[
	\Rp(w) = \min_{\eta \in [0, B]} \bar \Rp(w, \eta).
	\]
	%to restrict the minimization over $\eta$ to $[0, B]$.
	We define the analogous empirical version $\bar \Rpn(w, \eta)$ so that 
	$\Rpn(w) = \min_{\eta \in [0, B]} \bar \Rpn(w, \eta)$. 
	Note that $\bar \Rpn(w, \eta)$ is measurable for each fixed $(w, \eta)$ and $\Rpn(w)$ is measurable for each fixed $w$.
	
	\textit{Claim 1: Under Assumption\;\ref{assump:loss}, the random variable 
	\[
	\delta_n(w, \eta) := \bRpn(w, \eta) - \bar \Rp(w, \eta)
	\]
	has mean zero, lies almost surely in $[-B, B]$, and satisfies}
	\begin{align} \label{eq:lipschitz}
		|\delta_n(w, \eta) - \delta_n(w', \eta')|
		\le 2M/(1-p) \dist_\varphi(w, w') + 2(1+1/(1-p)) |\eta - \eta'| \,.
	\end{align}
	Note first that $\mathbb{E}[\bRpn(w, \eta)] = \bar \Rp(w, \eta)$
	and that the boundedness of $\delta_n$ comes from the boundedness of the loss function. 
	%Let us prove now that 
	The Lipschitzness of $\delta_n$ also comes from the one of the loss function, as follows.
	Using that $\max\{\cdot, 0\}$ is $1$-Lipschitz and that the loss $\ell$ is 
	$M$-Lipschitz, we get 
	\begin{align}
		|\max\{\ell(y, \varphi(w, x)) - \eta, 0\} 
			-& \max\{\ell(y, \varphi(w', x)) - \eta', 0\}|
		\\
		&\le |\ell(y, \varphi(w, x)) - \ell(y, \varphi(w', x))| 
		 	+ |\eta - \eta'| \\
        &\le M \|\varphi(w, x) - \varphi(w', x)\| + |\eta - \eta'| \\		 	
		&\le M\dist_\varphi(w, w') + |\eta - \eta'| \,.
	\end{align}
	Then, \eqref{eq:lipschitz} simply follows from the triangle inequality, and Claim 1 is proved. 
	
   \medskip
    The next step in the proof is, for a given  $\varepsilon > 0$ 
    \begin{itemize}
        \item to construct a cover $T$ of $W \times [0, B]$, and then 
        \medskip
        \item to control the convergence over the points of $T$, more precisely to control the probability of the event
        \[
		E_n(\varepsilon) = \bigcap_{(w, \eta) \in T} \left\{ \delta_n(w, \eta) \le \varepsilon / 2 \right\} \,.
	    \]
    \end{itemize}  %$E_n(\varepsilon)$ denote the event 
    
    First, using Assumption\;\ref{assump:cover}, we consider 
	$T_1$ a $(\varepsilon(1-p)/(8M))$-cover of $W$ with 
	respect to $\dist_\varphi$. We also consider $T_2$ a uniform discretization of the line segment $[0, B]$ at width $\varepsilon(1+1/(1-p))/8$. We can introduce the cover of $W \times [0, B]$ 
	\[
	T = T_1 \times T_2 \subset W \times [0, B]. %\qquad\text{which is a }
	\]
	Since, $|T_2| = 8B/((1+1/(1-p))\varepsilon)$, we have that 
	$|T| = (8B/((1+1/(1-p))\varepsilon)) \covnum(\varepsilon(1-p)/(8M))$.
	 Note that the event $\left\{ \delta_n(w, \eta) \le \varepsilon / 2 \right\}$ for fixed $(w, \eta)$ since $\delta_n(w, \eta)$ is measurable, and therefore, 
    $E_n(\varepsilon)$ is measurable since it is a finite intersection.

    To get uniform convergence, it is sufficient to control what happens at points of\;$T$. Indeed, for any $(w, \eta)$, there exists a point $(w', \eta') \in T$ such that $\dist_\varphi(w, w') \le \varepsilon(1-p)/(8M)$ and $|\eta - \eta'| \le \varepsilon (1+1/(1-p))/ 8$. As a consequence, if the event $E_n(\varepsilon)$ holds, then 
	\begin{align}
		\delta_n(w, \eta)
		&\ \le \delta_n(w', \eta') + 
			|\delta_n(w, \eta) - \delta_n(w', \eta')| \\
		&\stackrel{\eqref{eq:lipschitz}}{\le} 
			\delta_n(w', \eta') + 
			%2M \dist_\varphi(w, w')	+ 2 | \eta - \eta'| \\
			2M/(1-p) \dist_\varphi(w, w') + 2(1+1/(1-p)) | \eta - \eta'|\\
		&\ \le \frac{\varepsilon}{2} + \frac{\varepsilon}{4} + \frac{\varepsilon}{4}
		= \varepsilon.
	\end{align}
	
	This implies that events of interest are included in
	$\overline{E}_n(\varepsilon)$, the complement of $E_n(\varepsilon)$; we have indeed
	\[
	\left\{\sup_{w \in W} \, |\Rpn(w) - \Rp(w)| > \varepsilon\right\}
	\subset
	\left\{\sup_{(w,\eta) \in W \times [0, B]} \,  \delta_n(w, \eta) >\varepsilon\right\}
	\subset \overline E_n(\varepsilon)\,.
	\]
	Postponing the proof of measurability of these events to Claim 3 at the end of this proof, we have the following bound on the sum of probabilities
	%We finally get %for every $\varepsilon > 0$
	\begin{equation}\label{eq:finite}
	    \sum_{n=1}^\infty 
	    \mathbb{P}\Big(\sup_{w \in W }
	    \, |\Rpn(w) - \Rp(w)| > \varepsilon\Big)
	   % &\le 
	   % \sum_{n=1}^\infty \mathbb{P}\Big(\exists (w, \eta) \in W \times [0, B] \, :\, |\bar R_n(w, \eta) - \bar R(w, \eta)| > \varepsilon \Big)  \\
	    \le 
	    \sum_{n=1}^\infty \mathbb{P}\big(\overline E_n(\varepsilon)\big).
	\end{equation}

    \textit{Claim 2: The probabilities of the complements of $E_n(\varepsilon)$ are summable, i.e.,}
    \[
	\sum_{n=1}^\infty \mathbb{P}\big(\overline E_n(\varepsilon)\big)  < \infty \,.
	\]
	This is a direct application of the 
	Hoeffding's inequality (see e.g.~\cite[Theorem 2.2.2]{vershynin2018high})
% 	Hoeffding's inequality~\cite{hoeffding1963probability}, 
	as follows. For any fixed $(w, \eta) \in W \times [0, B]$, the Hoeffding's inequality gives 
	\[
		\mathbb{P}(|\delta_n(w, \eta)| > \varepsilon/2) \le
		2 \exp\left(- \frac{n\varepsilon^2}{2B^2}\right) \,.
	\]
	Applied to %the union over 
	all $(w, \eta) \in T$, this yields
	\[
		\mathbb{P}\big(\overline E_n(\varepsilon)\big) \le 
		2|T|\exp\left(- \frac{n\varepsilon^2}{2B^2}\right)
		= \frac{16B}{((1+1/(1-p))\varepsilon} \,
		\covnum\left(\frac{\varepsilon(1-p)}{8M}\right) \exp\left(- \frac{n\varepsilon^2}{2B^2}\right) \,.
	\]
    and proves Claim 2. 
   
\medskip

We conclude on the uniform convergence \eqref{eq:key} with the Borel-Cantelli Lemma by the classical rationale (see e.g.\;the textbook \cite[Chap.\;2, Sec.\;6]{pollard2002user}): the bound \eqref{eq:finite} and Claim 2 give that the probabilities for any $\epsilon$ are summable; applying Borel-Cantelli with the sequence $\epsilon_k=1/k$ gives the uniform convergence \eqref{eq:key}, which completes the proof of the theorem.

Finally, it remains to show measurability of some events of interest.

\textit{Claim 3: The following events are measurable for each $\varepsilon > 0$:}
\begin{align}
	E'_n(\varepsilon) &:= \left\{\sup_{w \in W} \, |\Rpn(w) - \Rp(w)| > \varepsilon\right\} \,,  \\
    E''_n(\varepsilon) &:= 
	\left\{\sup_{(w,\eta) \in W \times [0, B]} \,  \delta_n(w, \eta) >\varepsilon\right\} \,.
\end{align}

We prove the claim for $E'_n(\varepsilon)$ and the second one is entirely analogous. Since 
the set $\mathbb{Q}^d$ of $d$-dimensional rationals is dense in $\R^d$ and the map $w \mapsto |\Rpn(w) - \Rp(w)|$ is continuous, we have that 
\[
    \sup_{w \in W} \, |\Rpn(w) - \Rp(w)| = 
    \sup_{w \in W \cap \mathbb{Q}^d} \, |\Rpn(w) - \Rp(w)| \,.
\]
%The proof is completed by noting that 
Since the latter term is a supremum
%of countable set $\{ |\Rpn(w) - \Rp(w)|\, : \,  w \in W \cap \mathbb{Q}^d\}$ of measurable random variables.
over a countable set of measurable random variables, we get that $E'_n(\varepsilon)$ is measurable.

%===================================================================
%===================================================================
\section{Numerical Illustrations} \label{sec:a:Numerical Illustration}
%===================================================================
%===================================================================

We provide simple illustrations of the interest of using superquantile for machine learning. More precisely, we reproduce the experimental framework of the computational experiments of \cite{DBLP:conf/nips/CuriLJ020} and we solve the superquantile optimization problems with the approach depicted here, by combining smoothing and quasi-Newton. For additional experiments with other datasets, metrics, and contexts, we refer to \cite{DBLP:conf/nips/CuriLJ020}.

We consider two basic machine learning tasks (regression and classification) with linear prediction functions $\varphi(\x,x )=\trans{\x}x$ and with two standard datasets, from the UCI ML repository. Denoting these datasets $\Pn= \{(x_i,y_i)\}_{1 \leq i \leq n}$, we introduce the (regularized) empirical risk minimization 
% \[
% \min_{\x \in \Rd}
% ~~\mathbb{E}_{(x,y)\sim\Pn}\left[\ell(y, \trans{\x}x)\right] %\varphi(\x,x )\right] 
% +\frac{1}{2n}\norm{\x}^2\, ,
% \]
\[
\min_{\x \in \Rd}
~~\mathbb{E}_{(x,y)\sim\Pn}\left[\ell(y, \trans{\x}x)\right] %\varphi(\x,x )\right] 
+\frac{1}{2n}\|\x\|^2\, ,
\]
and its smoothed superquantile analogous
\[
\min_{\x \in \Rd} 
~~{[\Spnu]}_{(x,y)\sim\Pn}\left[\ell(y, \trans{\x}x) \right]
+\frac{1}{2n}\|\x\|^2\, .
\]
%where %For both models, 
%the regularisation parameter is set to $\lambda=1/n$.
%1/\text{n\_train} = 1/3341$. 

We solve these problems using L-BFGS via the toolbox \texttt{SPQR}~\cite{laguel2020first} offering an simple user-interface and implementing the oracles (with the Euclidean smoothing of Example\;\ref{ex:l2} for the smoothed approximation).

\begin{figure}[h!]
\begin{center}
  \includegraphics[width=7cm]{./images/abalone_regression.pdf}
\vspace*{-2ex}
  \caption{Regression: histogram of the regression errors on the testing dataset for the model learning by the superquantile approach (red) compared to the one of the classical empirical risk minimization (violet). We see a reshaping of the histogram of errors and a gain on worst-case errors.\label{fig:abalone}}
 \end{center}
\end{figure}

\medskip
%===================================================================
\textbf{Regression and Least-Squares}

We consider a regularised least square regression on the dataset Abalone from the UCI Machine learning repository.
We perform a $80\%/20\%$ train-test split on the dataset.
We minimize the least-squares loss on the training set both in expectation and with respect to the superquantile (with $p=0.98$ and $\nu=0.1$). 

% The superquantile version a smooth approximation of the superquantile with the euclidean smoothing detailed in~\ref{ex:l2}. 
% The smoothing parameter used is $0.1$ and leads to a succesful termination of L-BFGS
%(We note that two small values tend to cause an crash of the line-search procedure of BFGS).
We report on Figure~\ref{fig:abalone} the distribution of errors $|y_i - \trans{\x}x_i|$ for the testing dataset for both models $\x$ (standard in blue and superquantile in red). We observe that the superquantile model exhibits a thinner upper tail than the risk-neutral model, which is quantified by the shift to the left of $0.98$ quantile. This comes at the price of lower performance in expectations than the model trained with expectation, which is clear visible on the picture and quantified by the shift to the right of the mean.

\medskip
%===================================================================
\textbf{Classification and Logistic regression} 

We consider a logistic regression on the Australian Credit dataset. We randomly split the dataset with a $80\%/20\%$ train-test split for 5 different seeds. For each seed, we perform a pessimistic distributional shift on the training dataset by downsampling the majority class (similarly to what is done in \cite[Sec.\;5.2]{DBLP:conf/nips/CuriLJ020}). More precisely, we remove an important fraction of the majority class, randomly selected, so that it counts afterward for only $10\%$ of the minority class. We tune then the safety level parameter p by a k-cross validation on the shifted dataset and select the safety parameter yielding the best validation accuracy. The grid we use for tuning this parameter is [0.8, 0.85, 0.9, 0.95, 0.99]
We finally compute with this parameter the testing accuracy and the testing precision.

We report the testing accuracy and the testing precision averaged over the 5 different seeds on the table of Figure\;\ref{tab:table} with the associated standard deviation. 
We observe that the superquantile model brings better performance for both in terms of accuracy and precision than the standard model.

\begin{figure}[h!]
\begin{center}
  \begin{tabular}{ccc} \hline
  Model & Accuracy & Precision  \\ \hline
  Standard & $0.65\pm 0.03$ & $0.56\pm 0.04$ \\ 
  Superquantile & $0.69\pm 0.04$ & $0.60\pm 0.05$\\ \hline
  \end{tabular}
 \vspace*{-1ex}
  \caption{Classification: better testing accuracy and precision for the superquantile approach, in the case of distributional shifts.\label{tab:table}}
  \end{center}
\end{figure}

% \begin{figure}
% \begin{floatrow}
% \ffigbox{%
%   \vspace*{-1ex}
%   \centerline{\includegraphics[width=5.5cm]{./images/abalone_regression.pdf}}
% \vspace{-1ex}
% }{%
%   \caption{Risk-averse regression on Abalone}\label{fig:abalone}
% }
% \capbtabbox{%
% \begin{center}
%   \begin{tabular}{ccc} \hline
%   Model & Accuracy & Precision  \\ \hline
%   Expectation & $0.65\pm 0.03$ & $0.56\pm 0.04$ \\ 
%   Superquantile & $0.69\pm 0.04$ & $0.60\pm 0.05$\\ \hline
%   \end{tabular}
%  \end{center}
% }{%
%   \caption{Distributionally robust logistic regression on the Australian credit dataset}%
% }
% \end{floatrow}
% \end{figure}

% \begin{figure}
% \begin{floatrow}
% \ffigbox{%
%   \vspace*{-1ex}
%   \centerline{\includegraphics[width=5.5cm]{./images/abalone_regression.pdf}}
% \vspace{-1ex}
% }{%
%   \caption{Superquantile\;regression} %: superquantile vs stan}%
% }
% \capbtabbox{%
%  \vspace*{-10ex}
% \begin{center}
%  %\vspace*{-10ex}
%   \begin{tabular}{ccc} \hline
%   Model & Accuracy & Precision  \\ \hline
%   Expectation & $0.65\pm 0.03$ & $0.56\pm 0.04$ \\ 
%   Superquantile & $0.69\pm 0.04$ & $0.60\pm 0.05$\\ \hline
%   \end{tabular}
%  \end{center}
%   \vspace*{8ex}
% }{%
%   \caption{Superquantile\;classification}%
% }
% \end{floatrow}
% \end{figure}
